# Supplementary material for: Conditional Generation with a Question-Answering Blueprint
Source: arXiv:2207.00397 source file (2023-05-01)
Supplement: Supplementary file 1 [file human-eval-results-appendix.tex]

\begin{table}[t!]
\center
% \scriptsize
%\tiny
\resizebox{\linewidth}{!}{
{\setlength{\tabcolsep}{0pt}%
\begin{tabular}{l@{}|@{~} c|@{~} c@{~~} c @{~}|@{~} c@{~~} c@{~~} c@{}} \hline
& summary & \multicolumn{2}{c@{~}|@{~}}{blueprint} &  \multicolumn{3}{c@{~}@{~}}{grounding} \\
% & \multicolumn{2}{c@{~}|@{~}}{Rouge (RLSum)} &  \multicolumn{2}{c|@{~}}{QA-F1} & \multicolumn{1}{c}{ANLI}  \\ 
& best & quality & redund.& abs. & contr. & new-info \\ 
Models & 0-to-1 & 1-to-3 & \% & \% & \% & 3-to-1 \\ \hline 
\textsc{SiBERT} & 0.12 & --- & --- & --- & --- & \multicolumn{1}{c}{---}  \\  
\longtv & \textbf{0.49} & --- & --- & --- & --- & \multicolumn{1}{c}{---}  \\  
\cellcolor{DarkBP}\textcolor{white}{\etoe} & 0.39$^{\diamond}$ & \textbf{2.83} & \textbf{8.3}$^{\diamond}$ & 6.3$^{\diamond}$ & 4.1$^{\diamond}$ & 1.79$^{\diamond}$ \\
\cellcolor{DarkBP}\textcolor{white}{\aplan} & 0.39$^{\diamond}$ & 2.58$^{\diamond}$ & 16.0$^{\diamond}$ & 13.2 & 13.6 & 2.06 \\
\cellcolor{DarkBP}\textcolor{white}{\iterative} & 0.30$^{\dagger}$ & 2.51$^{\diamond}$ & 40.0$^{\dagger}$ & 5.0$^{\diamond}$ & 2.5$^{\diamond}$ & \textbf{1.77}$^{\diamond}$ \\
\hspace{0.2cm} \cellcolor{MidBP}\textcolor{white}{+drop} & 0.31$^{\dagger}$ & 2.56$^{\diamond}$ & 36.7$^{\dagger}$ & \textbf{4.9}$^{\diamond}$ & \textbf{2.3}$^{\diamond}$ & 1.86$^{\diamond}$ \\
\hline
Gold & --- & 2.85 & 7.0 & 3.6 & 2.4 & 1.88 \\ \hline
\end{tabular}}
}
  \vspace{-0.2cm}
\caption{\sn{} Human evaluation results on Aquamuse query-focused summarization. The best results for each task are \textbf{boldfaced}. 
Systems in each column are marked with same symbols when differences among them are not significant (using a one-way ANOVA with post-hoc Tukey HSD tests; $p < 0.01$).    \label{table:heval-results-aquamuse} }
    \vspace{-0.6cm}
\end{table}

\begin{table}[t!]
\center
% \scriptsize
%\tiny
\resizebox{\linewidth}{!}{
{\setlength{\tabcolsep}{0pt}%
\begin{tabular}{l@{}|@{~} c|@{~} c@{~~} c @{~}|@{~} c@{~~} c@{~~} c@{}} \hline
& summary & \multicolumn{2}{c@{~}|@{~}}{blueprint} &  \multicolumn{3}{c@{~}@{~}}{grounding} \\
% & \multicolumn{2}{c@{~}|@{~}}{Rouge (RLSum)} &  \multicolumn{2}{c|@{~}}{QA-F1} & \multicolumn{1}{c}{ANLI}  \\ 
& best & quality & redund.& abs. & contr. & new-info \\ 
Models & 0-to-1 & 1-to-3 & \% & \% & \% & 3-to-1 \\ \hline 
% \textsc{r2t-Bart} &  & --- & --- & --- & --- & \multicolumn{1}{c}{---}  \\  
\longtv & 0.35$^{\diamond}$ & --- & --- & --- & --- & \multicolumn{1}{c}{---}  \\  
\cellcolor{DarkBP}\textcolor{white}{\etoe} & 0.40$^{\dagger}$ & \textbf{2.94}$^{\diamond}$ & \textbf{4.7}$^{\diamond}$ & \textbf{2.0}$^{\diamond}$ & \textbf{0.4}$^{\dagger}$ & \textbf{1.74}$^{\diamond}$ \\
\cellcolor{DarkBP}\textcolor{white}{\aplan} & 0.37$^{\diamond\dagger}$ & 2.84$^{\diamond}$ & 6.3$^{\diamond}$ & 5.8$^{\dagger}$ & 3.7$^{\diamond}$ & 1.91$^{\dagger}$ \\
\cellcolor{DarkBP}\textcolor{white}{\iterative} & 0.28$^{\ddagger}$ & 2.64$^{\dagger}$ & 31.0$^{\dagger}$ & 2.8$^{\diamond}$ & 2.9$^{\diamond}$ & \textbf{1.74}$^{\diamond}$ \\
\hspace{0.2cm} \cellcolor{MidBP}\textcolor{white}{+drop} & 0.27$^{\ddagger}$ & 2.66$^{\dagger}$ & 27.3$^{\dagger}$ & 3.6$^{\diamond\dagger}$ & 2.1$^{\dagger\diamond}$ & 1.90$^{\dagger}$ \\
\hline
Gold & --- & 2.67 & 14.3 & 1.6 & 1.8 & 2.02 \\ \hline
\end{tabular}}
}
  \vspace{-0.2cm}
\caption{\sn{} Human evaluation results on WikiCatSum multidocument summarization. The best results for each task are \textbf{boldfaced}. 
Systems in each column are marked with same symbols when differences among them are not significant (using a one-way ANOVA with post-hoc Tukey HSD tests; $p < 0.01$).    \label{table:heval-results-wikicatsum} }
    \vspace{-0.6cm}
\end{table}

% $^{\ddagger}$
% $^{\diamond}$

% Tukey HSD results
% treatments
% pair	Tukey HSD
% Q statistic	Tukey HSD
% p-value	Tukey HSD
% inferfence
% A vs B	4.5579	0.0111535	* p<0.05
% A vs C	2.1959	0.5241464	insignificant
% A vs D	5.8951	0.0010053	** p<0.01
% A vs E	7.4674	0.0010053	** p<0.01
% B vs C	2.3613	0.4544029	insignificant
% B vs D	10.4501	0.0010053	** p<0.01
% B vs E	12.0226	0.0010053	** p<0.01
% C vs D	8.0888	0.0010053	** p<0.01
% C vs E	9.6610	0.0010053	** p<0.01
% D vs E	1.5710	0.7748900	insignificant
